# Supplementary material for: Progressive Supervision via Label Decomposition: An Long-Term and Large-Scale Wireless Traffic Forecasting Method
Source: arXiv:2501.06255 source file (2025-01-09)
Supplement: Supplementary file 1 [file appendixes.tex]

\section*{Appendix}
\label{sec_app}

Now we give proof of the representation ability of RSS.

\begin{proof}
Let $A(v)$ denote the true aggregated feature for node $v$ using the entire graph:
\begin{equation}
A(v) = \sum_{u \in N(v)} \frac{1}{C_{vu}} Wh_u,
\end{equation}
where $N(v)$ is the set of neighbors of $v$, $h_u$ is the feature of node $u$, 
$C_{vu}$ is a normalization constant, $W$ is the weight matrix.
For the sampled subgraph $G'$, the aggregated feature $A'(v)$ is given by:
\begin{equation}
  A'(v) = \sum_{u \in N(v) \cup V'} \frac{1}{C_{vu}P(u)} Wh_u,
\end{equation}
where $P(u)$ is the probability of node $u$ being sampled.
To show that $A'(v)$ is an unbiased estimator of $A(v)$, we compute the expectation of $A'(v)$:
\begin{equation}
  \mathbb{E}[A'(v)] = \mathbb{E}\left[ \sum_{u \in N(v) \cup V'} \frac{1}{C_{vu}P(u)} Wh_u \right].
\end{equation}
Since nodes are sampled independently, we can write:
\begin{equation}
  \mathbb{E}[A'(v)] = \mathbb{E}\left[ \sum_{u \in N(v)} \frac{\mathbb{I}(u\in V')}{C_{vu}P(u)} Wh_u \right],
\end{equation}
where $\mathbb{I}(u\in V')$ is an indicator function that is $1$ if 
$u$ is sampled and $0$ otherwise. The expectation of the indicator function is simply the probability of sampling $u$: $\mathbb{E}[\mathbb{I}(u\in V')]=P(u)$. Thus, 
\begin{align}
  \mathbb{E}[A'(v)] &= \sum_{u \in N(v)} \mathbb{E}\left[ \frac{\mathbb{I}(u\in V')}{C_{vu}P(u)} Wh_u \right] \notag \\
  &= \sum_{u \in N(v)} \frac{P(u)}{C_{vu}P(u)} Wh_u \notag \\
  &= \sum_{u \in N(v)} \frac{1}{C_{vu}} Wh_u. 
\end{align}
This shows that the expected aggregated feature using RSS is an unbiased estimator of the true aggregated feature using the entire graph.
\end{proof}
